# Supplementary material for: Tune: A Research Platform for Distributed Model Selection and Training
Source: arXiv:1807.05118 source file (2018-07-13)
Supplement: Supplementary file 1 [file appendix.tex]

\section{Algorithm Families}
\label{sec:app_survey}

\textbf{Policy Gradients}: This family of algorithms such as Vanilla Policy
Gradient \cite{williams1992simple}, TRPO \cite{schulman2015trust,
schulman2015gae}, PPO \cite{schulman2017proximal} commonly utilize policy
evaluation and gradient-based optimization in two separate phases, abiding to
the generalized policy iteration model \cite{sutton1998reinforcement}. Some
algorithms such as A3C \cite{mnih2016asynchronous} execute the two
simultaneously.

\textbf{Deep Q-Networks:} Most DQN variants \cite{bellemare2017distributional,
hessel2017rainbow, mnih2015human, schaul2015prioritized, van2016deep,
wang2015dueling} use a gradient-based optimizer to update the policy, but they
additionally utilize a replay buffer as an off-policy data source.

\textbf{Policy Gradient with Off Policy:} These algorithms, such as DDPG
\cite{lillicrap2015continuous}, Q-Prop \cite{gu2016q}, ACER
\cite{wang2016sample}, UNREAL \cite{jaderberg2016reinforcement} are extensions
of an existing policy gradient method such as A3C that utilize an off policy
data source such as a replay buffer to augment the training process.

\textbf{Model-Based:} This includes Model-Based combined with Model-Free
learning. This family of algorithms, including I2A \cite{weber2017imagination},
IBP \cite{pascanu2017learning}, Value Prediction Networks \cite{oh2017value},
augments policy evaluation as a planning subroutine to inform the policy during
a rollout.

\textbf{Multi-Agent RL:} Modern approaches in this area \cite{lowe2017multi,
foerster2016learning, mordatch2017emergence, peng2017multiagent} tend to use
gradient-based optimizers along with parallel policy evaluation from each agent
to collect data and update the policy. Experience replay
\cite{foerster2017stabilising} has also been considered in this setting.

\textbf{Evolutionary Methods:} Methods such as Evolutionary Strategies
\cite{salimans2017evolution} and Covariance Matrix Adaptation
\cite{hansen1996adapting} tend to rely on Derivative Free Optimization and Monte
Carlo methods instead of Gradient Based Optimization.

In addition to these broader areas of RL, we also consider the design of
large-scale RL systems:

\textbf{AlphaGo:} AlphaGo Zero \cite{silver2017mastering} utilizes multiple
parameter servers feeding from a replay buffer, updated from a self-play agent
evaluating the best current policy.

\section{Evolutionary Composition Case Study}

\begin{figure}[h]
  \centering
  \begin{subfigure}[PPO-ES]{
      \includegraphics[width=6cm]{fig/walker2d.pdf}
  }
  \end{subfigure}
  \begin{subfigure}[A3C-ES]{
      \includegraphics[width=6cm]{fig/hierA3C.pdf}
  }
  \end{subfigure}

  \caption{Evolutionary variants of PPO and A3C outperform their base
  implementations on Walker2d-v1 and PongDeterministic-v4 environments
  respectively. PPO-ES also converged to a higher reward.}

  \label{figure:ppoes}
\end{figure}

\section{Choosing the right SGD strategy}
\label{sec:rloptimizer}

Deep learning frameworks perform many internal optimizations such as operator
fusion \cite{nnvm, abadi2017computational}. However, in many RL workloads data
transfers across non-differentiable graph boundaries (e.g. during simulation)
incur significant overheads. In the cluster setting, the right physical strategy
for RL optimization can vary depending on factors including:

\begin{enumerate}[wide, labelwidth=!, labelindent=8pt]

  \item \textbf{Resource availability}: It may be cost prohibitive to provision
  GPU devices on each node in a large compute cluster. In this case, it may
  makes sense to send sample data to nodes with GPUs. Alternatively, a
  large number of CPUs may be just as fast, e.g. as in A3C.

  \item \textbf{Relative data sizes}: If sample data is small relative to
  the model, it may be more efficient to send samples to the driver for
  SGD. Conversely if samples are large, network traffic is minimized by
  keeping them local to worker processes.

  \item \textbf{Algorithm}: Algorithm-specific details can often be exploited.
  For example, PPO's loss function permits multiple SGD passes. Table
  \ref{table:sgd_tradeoffs} shows how this can be exploited in certain cases to
  amortize CPU-to-GPU copy costs, increasing SGD throughput by 6x.

\end{enumerate}

\RLLib{} chooses an initial SGD strategy based on simple algorithm and
environment-specific heuristics. Thanks to the task-based programming model, it
can also adaptively switch strategies based on runtime statistics (Figure
\ref{fig:a3c_tradeoffs}).

\begin{figure*}[ht!]
  \centering
  \begin{subfigure}[Gradient latency history, CPU-only]{
      \includegraphics[width=6cm]{fig/sgd_no_gpu_timing.pdf}
  }
  \end{subfigure}
  \hspace{1cm}
  \begin{subfigure}[Gradient latency history with GPU driver]{
      \includegraphics[width=6cm]{fig/sgd_gpu_timing.pdf}
  }
  \end{subfigure}

    \caption{\RLLib{} can adaptively identify the best SGD strategy, switching
    to the optimal choice within a few iterations. Here the optimal strategy for
    A3C (computing gradients on the driver vs on remote workers) changes
    depending on whether the driver has access to a GPU.}

  \label{fig:a3c_tradeoffs}
\end{figure*}

\section{Evaluation Hyperparameters}
\label{sec:hyperparameters}

\subsection{Hyperparameters for Evolution Strategies}

\begin{table}[h]
\begin{center}
\begin{tabular}{l | l}
{\bf Hyperparameter} & {\bf Value} \\\hline
Noise standard deviation & 0.02\\
Adam stepsize & 0.01\\
L2 coefficient & 0.005\\
Episodes per batch & 5000\\
\end{tabular}
\end{center}
\end{table}

\subsection{Hyperparameters for Proximal Policy Optimization}

\begin{table}[h]
\begin{center}
\begin{tabular}{l | l}
{\bf Hyperparameter} & {\bf Value} \\\hline
Timesteps per batch & 320000\\
SGD minibatch size & 32768\\
SGD epochs per iteration& 20\\
Adam stepsize & 1e-4\\
PPO clip param & 0.2\\
GAE parameter ($\lambda$) & 0.95\\
Discount ($\gamma$) & 0.995\\
\end{tabular}
\end{center}
\end{table}

\section{Case Study Pseudocode}
\label{sec:case_study_code}

\subsection{Offline Data Evaluator}
\label{subsec:offline_eval_code}
\verbatiminput{code/offline_evaluator.py}

\subsection{PPO-ES}
\label{subsec:ppoes_code}
\verbatiminput{code/ppoes.py}

\subsection{AlphaGo Zero}
\label{subsec:alphago_zero_code}
\verbatiminput{code/alphago.py}

\subsection{Hyperparam Search Integration}
\label{subsec:hyperparam_search_code}
\verbatiminput{code/hyperparam_integration.py}
